# Supplementary material for: Three-Dimensional Reconstruction of Weak Lensing Mass Maps with a Sparsity Prior. I. Cluster Detection
Source: arXiv:2102.09707 source file (2022-02-02)
Supplement: Supplementary file 1 [file appendix.tex]

%Intro

The primary goal of most weak-lensing surveys is to constrain the cosmology
model through the $2$-point correlations. The studies include galaxy$-$galaxy
lensing, which cross-correlating the shear field ($\gamma$) with the positions
of foreground galaxies
\citep{gglens-GAMA-Han2014,gglens-BossCFHTMore2015,gglens-DES1}, and cosmic
shear which auto-correlates the shear measurements
\citep{cosmicShearRealKids450,cosmicShear-DES1,cosmicShear_HSC1_Chiaki2019,cosmicShear_HSC1_Hamana2019}.
Since the shear is directly related to the foreground matter distribution as
shown in eq. (\ref{eq-intro-delta2shear}), Galaxy$-$galaxy lensing probes into
the correlation between the matter field and galaxy field. On the other hand,
cosmic shear probes into the auto-correlation of matter field.

% weak lensing
The lensing convergence to the comoving distance $\chi_s$ is contributed by the
foreground inhomogeneous density distribution as
\begin{equation}
\kappa(\vec{\theta},\chi_s)=\frac{3H_0^2\Omega_{\rm m}}{2 c^2} \int_0^{\chi_s} d\chi_l \,
\frac{\chi_l \chi_{sl}}{\chi_s}
\frac{\delta(\vec{\theta},\chi_l)}{a(\chi_l)},
\end{equation}
where $\delta=\rho(\vec{\theta},\chi_l)/\bar{\rho}-1$ is the density contrast
at the position of lens, $c$ is the speed of light, $\chi_{sl}$ is the comoving
distance between source and lens plane, and $a(\chi_l)$ is the scale parameter
at the lens position.

The corresponding convergence to redshift $z_s$ is
\begin{equation}\label{eq-delta2kappa}
\kappa(\vec{\theta},z_s)=\int_0^{z_s} \,dz_l \,K(z_l,z_s)\,\delta(\vec{\theta},z_l).
\end{equation}

Following \citet{massMap-KS1993}, we relate the shear field to the kappa
field at the same source redshift by
\begin{equation}\label{eq-kappa2gamma}
\gamma_L(\vec{\theta},z_s) = \int  d^2 \theta' D(\vec{\theta}-\vec{\theta'})\, \kappa(\vec{\theta'},z_s),
\end{equation}
where

Here we denote the physical shear distortion as $\gamma_L$, which is {\it not}
the final shear measurement since shear measurement is influenced by systematic
errors in observations. The relevant systematic errors will be discussed in
detail in Section \ref{subsec_method_Systematics}.

Combining eq. (\ref{eq-delta2kappa}) with eq. (\ref{eq-kappa2gamma}), the
expectation of lensing shear signal is
\begin{equation}\label{eq-delta2gammat}
\gamma_L(\vec{\theta},z_s) = \int_0^{z_s} dz_l K(z_l,z_s)
\int d^2 \theta' \vec{D}(\vec{\theta}-\vec{\theta'}) \delta(\vec{\theta'},z_l).
\end{equation}

To simplify the expression, we define the lensing transformation operator as
\begin{equation}
\mathbf{Q}=\int_0^{z_s} dz_l K(z_l,z_s) \int d^2 \theta'  \vec{D}(\vec{\theta}-\vec{\theta'}),
\end{equation}
and then eq. (\ref{eq-delta2gammat}) reduces to
\begin{equation} \label{eq-delta2gammat-simp}
\gamma_L=\mathbf{Q}\,\delta.
\end{equation}

From eqs.~\eqref{eq-delta2gamma} and \eqref{eq-x2delta}, we obtain the following
expression in linear operator form:
\begin{equation}\label{eq-x2gammat}
    \gamma=\mathbf{T}\,\mathbf{\Phi}\,x\,.
\end{equation}

% Sparsity

We assume that the halos are sparsely distributed in the universe.  With the
sparsity prior, the adaptive LASSO regularization \citep{AdaLASSO-Zou2006} can
be used to reconstruct the density field. We expect the adaptive LASSO to
reduce the smearing effect, in contrast to the ordinary LASSO estimator that
tends to smear the structure along line of sight
\citep{LSS-massMap-Glimpse3D-Leonard2014}. Furthermore, the adaptive LASSO
algorithm is strictly convex and can be directly optimized with the FISTA
algorithm \citep{FISTA-Beck2009} without relying on any greedy coordinate
descent approaches.
